# Supplementary material for: How Useful is Continued Pre-Training for Generative Unsupervised Domain Adaptation?
Source: arXiv:2401.17514 source file (2025-03-01)
Supplement: Supplementary file 1 [file sensitivity_analysis_experimental.tex]

\section{Learning with Larger Models}
\label{sec:appendix-more-results}

The use of high capacity language models, which are too compute intensive for traditional fine-tuning, originally encouraged the use of prompting, and prompting is now common with learning from large language models \cite{brown2020language, schick2021exploiting, schick2021s, gao2021making}.
Since our approach makes use of prompting, we investigate the performance of \mlm~with such models. 

We experiment with two large models: T5v1.1 XL (3 billion parameters) and T0 (3 billion parameters). T0 is optimized for zero-shot generalization by training on supervised prompts. We use the Apparel (A) $\to$ Movies (M) domain pair from the Amazon Reviews dataset.
Table~\ref{tab:varying-models} shows the performance gap between \mlm~and \mmd~increasing with larger models.
In the case of T0, we see particularly poor performance with \mmd. 
This may be due to the fact that the task of minimizing the divergence between embeddings is highly different from the tasks a model is trained on during instruction tuning.

\input{tables/performance_across_models}
